# Supplementary material for: Anomalous Tip-Sample Distance Behavior on the Tip-Enhanced Raman Spectroscopy of Graphene in Ambient Conditions
Source: arXiv:2601.14178 ancillary file (2026-01-20)
Supplement: Supplementary file 1 [file Anomalous_tip-sample_distance_behavior_SM.pdf]

# **Supplementary Material for Anomalous Tip-Sample Distance Behavior on the Tip-Enhanced Raman Spectroscopy of Graphene in Ambient Conditions**

André G. Pereira,<sup>1,2</sup> Raul Corrêa,<sup>1,3</sup> Bianca Carneiro,<sup>1</sup> Cassiano Rabelo,<sup>2</sup> Thiago L. Vasconcelos,<sup>4</sup> Vitor Monken,<sup>2,5</sup> Luiz Gustavo Cançado,<sup>1</sup> and Ado Jorio<sup>1</sup>

<sup>1)</sup>*Departamento de Física, Universidade Federal de Minas Gerais, Belo Horizonte, Minas Gerais, 30123-970 Brazil*

<sup>2)</sup>*FabNS, Parque Tecnológico de Belo Horizonte-BHTec, Belo Horizonte, Brazil*

<sup>3)</sup>*Instituto D'Or de Pesquisa e Ensino/Pioneer Science Initiative, Rio de Janeiro, RJ 22281-010, Brazil*

<sup>4)</sup>*Instituto Nacional de Metrologia, Qualidade e Tecnologia, Duque de Caxias, RJ 25250-020, Brazil*

<sup>5)</sup>*Programa de Pós-Graduação em Inovação Tecnológica e Propriedade Intelectual, Universidade Federal de Minas Gerais, Belo Horizonte, Brazil*

(Dated: 19 January 2026)

## I. CLASSIFICATION AND QUANTITATIVE ANALYSIS OF DECAY REGIMES

Here we present the decay curves together with the undeformed and deformed model curves, analyzing the normalized 2D band intensity. Two distinct behaviors can be identified:

(i) Without a regime change, corresponding to a single-phase decay, as shown in Figure 1a, characterized by a smooth and monotonic decrease in the TERS near-field intensity without any identifiable regime transition. This data is well adjusted by the undeformed model.

(ii) With a regime change, corresponding to a two-phase decay. In this case, the behavior can be further classified into two categories: a smooth transition between decay regimes (Figure 1b) and an abrupt, step-like transition (Figure 1c). The former will be referred to as continuous ( $C$ ), and the latter as discontinuous ( $D$ ) in the subsequent analysis. The deformed model provides an accurate description of the experimental behavior for both curves, including the abrupt step observed in the  $D$ -type curves. As one should expect, the abrupt transition is characterized by a small transition width ( $W_S$ ) compared to the continuous transition.

54 experiments were performed, and the classifications, following the definitions provided above, are presented in Table I.

TABLE I. Summary of the decay classifications obtained from the retract experiments.

| Decay Behavior | Transition | Number of experiments |
|----------------|------------|-----------------------|
| Single-phase   | -          | 10                    |
| Two-phase      | C          | 39                    |
| Two-phase      | D          | 5                     |

The deformation parameters vary throughout the experiments. Figure 2 presents histograms relating the number of experiments to the snap-out distance,  $W_S$  and  $\Delta S$ , for both continuous and discontinuous transitions. It is possible to conclude that the C transition is the more likely outcome, with the average snap-out events observed around 12.5 nm.

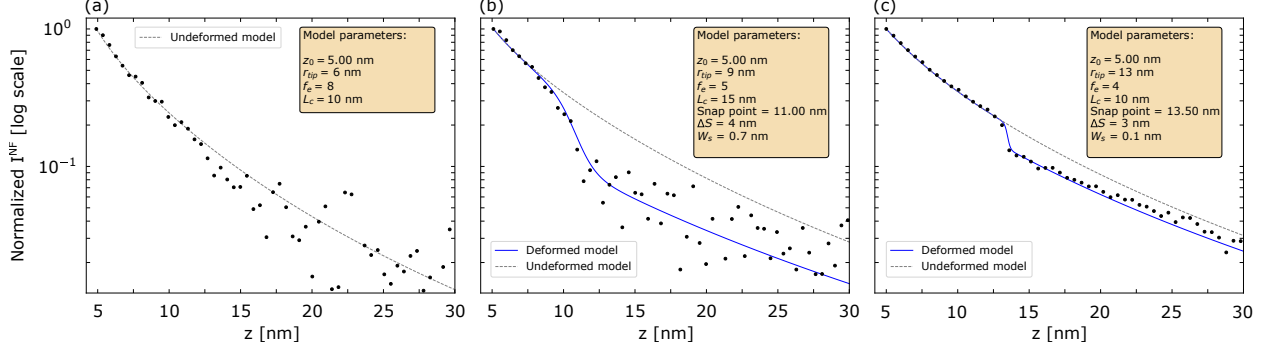

FIG. 1. Examples of (a) single-phase decay curve and two-phase decay curve with (b) continuous transition and (c) with discontinuous transition.

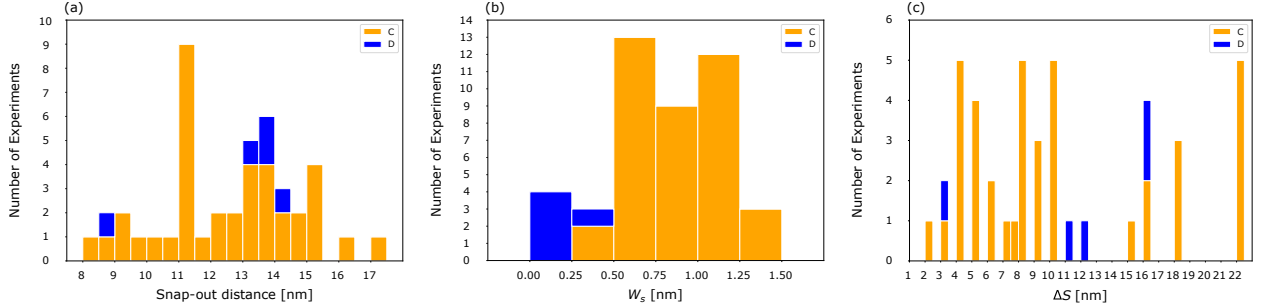

FIG. 2. Histograms showing the distribution of the deformation parameters: (a) snap-out distance, (b)  $W_s$ , and (c)  $\Delta S$ . The continuous transitions are shown in yellow and the discontinuous in blue.

## II. FREQUENCY VARIATION

Along with the amplitude, one of the returned parameters from the AFM-control is the frequency variation from the resonance frequency of the tuning fork, named  $\Delta F$ . Figure 3 depicts the TERS near-field intensity  $I^{NF}(z)$  decay along with the tuning fork frequency variation in the same two experiments shown in Figure 2 from the main text.

The main difference between the  $\Delta F$  and amplitude curves is that the frequency change is more pronounced at small  $z$  separations (approximately 6 nm) in both experiments. A slight variation in  $\Delta F$  is observable over a narrow range (6 nm to 8 nm) during approach, but over a much broader range (6 nm to 18 nm) during retraction. The final  $z$  separation where the frequency signal is dominated by noise coincides precisely with the snap-in and snap-out positions discussed in the main text.

One explanation for this behavior is that frequency variations ( $\Delta F$ ) are generally at-

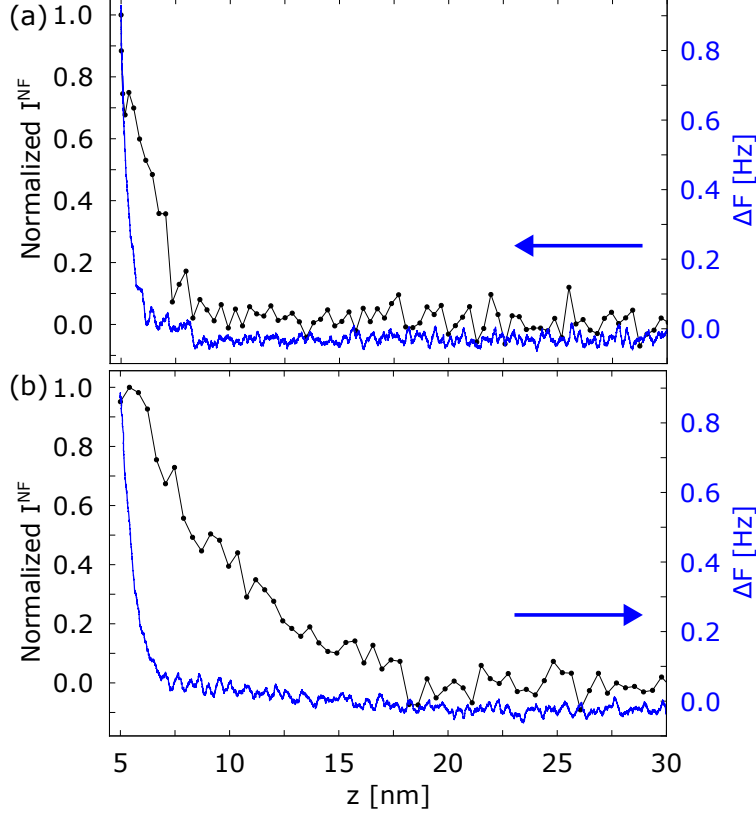

FIG. 3. Normalized TERS near-field intensity decay  $I^{NF}(z)$  alongside the corresponding tuning fork frequency variation ( $\Delta F$ ) for the approach (a) and retraction (b) experiments. The arrows indicate the direction of the tip movement. The  $\Delta F$  curves were smoothed using a Savitzky-Golay filter.

tributed to conservative forces. The steep decay observed in small  $z$  separations agrees with this principle, as the conservative forces that govern the tip-sample interaction are most significant at these smaller distances. Conversely, dissipative forces, such as the viscous drag present when the tuning fork oscillates inside the meniscus, are responsible for changes in the amplitude but have a minor effect on the vibration frequency.<sup>1</sup> This distinction explains why the changes in the amplitude curves persist at larger  $z$  separations, while the  $\Delta F$  changes do not.

## REFERENCES

<sup>1</sup>F. J. Giessibl, “Advances in atomic force microscopy,” Rev. Mod. Phys. **75**, 949–983 (2003).
